# Supplementary material for: Effects of spin-orbit coupling and in-plane Zeeman fields on the critical current in two-dimensional hole gas SNS junctions
Source: arXiv:2210.13266 source file (2023-02-02)
Supplement: Supplementary file 1 [file supplementary.pdf]

# Supplemental material for "2D hole gas Josephson junction"

Jonas Lidal and Jeroen Danon
*Center for Quantum Spintronics, Department of Physics,*
*Norwegian University of Science and Technology, NO-7491 Trondheim, Norway*
(Dated: May 5, 2022)

## I. PERTURBATIVE CALCULATION OF JOSEPHSON CURRENT

The current in the ground state is given by

$$J = \frac{2e}{\hbar}\frac{\partial F}{\partial \phi}, \tag{1}$$

where $\phi$ is the phase difference between the two superconductors and $F$ is the free energy of the junction, $F = E - \mu N$. The temperature Green functions are defined as

$$\begin{aligned}
\mathcal{G}_{\alpha\beta}(\mathbf{r}_1,\tau_1;\mathbf{r}_2,\tau_2) &= -\frac{1}{Z}\mathrm{Tr}\left\{e^{-\beta(\hat{H}-\mu\hat{N})}\hat{T}_\tau \psi_\alpha(\mathbf{r}_1,\tau_1)\psi^\dagger_\beta(\mathbf{r}_2,\tau_2)\right\} \\
&= -\frac{\mathrm{Tr}\left\{e^{-\beta(\hat{H}-\mu\hat{N})}\hat{T}_\tau \psi_\alpha(\mathbf{r}_1,\tau_1)\psi^\dagger_\beta(\mathbf{r}_2,\tau_2)\right\}}{\langle e^{-\beta\hat{H}}\rangle} \\
&= -\mathrm{Tr}\left\{e^{\beta F}e^{-\beta(\hat{H}-\mu\hat{N})}\hat{T}_\tau \psi_\alpha(\mathbf{r}_1,\tau_1)\psi^\dagger_\beta(\mathbf{r}_2,\tau_2)\right\} \\
&\equiv -\langle \hat{T}_\tau \psi_\alpha(\mathbf{r}_1,\tau_1)\psi^\dagger_\beta(\mathbf{r}_2,\tau_2)\rangle.
\end{aligned} \tag{2}$$

The wave functions are here defined in the Heisenberg picture,

$$\psi_\alpha(\mathbf{r},\tau) = e^{(\hat{H}-\mu\hat{N})\tau}\psi_\alpha(\mathbf{r})e^{-(\hat{H}-\mu\hat{N})\tau}, \tag{3}$$

$$\psi^\dagger_\alpha(\mathbf{r},\tau) = e^{(\hat{H}-\mu\hat{N})\tau}\psi^\dagger_\alpha(\mathbf{r})e^{-(\hat{H}-\mu\hat{N})\tau}, \tag{4}$$

and the angle brackets signifies the Gibbs statistical average

$$\langle \ldots \rangle = \mathrm{Tr}\left\{e^{\beta(F-\hat{H}+\mu\hat{N})}\ldots\right\}. \tag{5}$$

Going to the interaction picture we split the Hamiltonian from the Schrödinger picture in two parts, one exactly solvable part and a perturbation or interaction part.

$$\hat{H} = \hat{H}_0 + \hat{H}_1. \tag{6}$$

In this picture all operators gain time-dependence due to $H_0$ only,

$$\psi_\alpha(\mathbf{r},\tau) = e^{(\hat{H}_0-\mu\hat{N})\tau}\psi_\alpha(\mathbf{r})e^{-(\hat{H}_0-\mu\hat{N})\tau}, \tag{7}$$

$$\psi^\dagger_\alpha(\mathbf{r},\tau) = e^{(\hat{H}_0-\mu\hat{N})\tau}\psi^\dagger_\alpha(\mathbf{r})e^{-(\hat{H}_0-\mu\hat{N})\tau}, \tag{8}$$

etc. The so called S-matrix is defined by

$$\mathcal{S}(\tau) = \hat{T}_\tau \exp\left\{-\int_0^\tau d\tau'\,\hat{H}_1(\tau')\right\}. \tag{9}$$

Also, by definition we have,

$$e^{-\beta F} = \mathrm{Tr}\left\{e^{-\beta(\hat{H}-\mu\hat{N})}\right\}, \tag{10}$$

which, with the use of the definition of the S-matrix, we can write as,

$$\begin{aligned}
e^{-\beta F} &= \mathrm{Tr}\left\{e^{-\beta(\hat{H}_0-\mu\hat{N})}\mathcal{S}(\beta)\right\} \\
&= e^{-\beta F_0}\mathrm{Tr}\left\{e^{\beta(F_0-\hat{H}_0+\mu\hat{N})}\mathcal{S}(\beta)\right\} \\
&= e^{-\beta F_0}\langle \mathcal{S}(\beta)\rangle_0.
\end{aligned} \tag{11}$$

Where $\langle \ldots \rangle_0$ is the Gibbs statistical average over the unperturbed ground state. This can be used to write the free energy as

$$F = F_0 - T\ln\langle \mathcal{S}\rangle_0. \tag{12}$$

When calculating $\langle\mathcal{S}\rangle_0$ we should take into account all allowed diagrams, connected as well as disconnected. However it can be shown [? ] that all diagrams can be expressed in terms of connected diagrams only. Defining the fully connected part of $\langle\mathcal{S}\rangle_0$ as

$$\langle\mathcal{S}\rangle_{\rm con} = 1 + \Xi_1 + \Xi_2 + \dots, \tag{13}$$

with $\Xi_n$ representing all $n$th order connected diagrams. The S-matrix for all connected and unconnected diagrams can be written in these as

$$\langle\mathcal{S}\rangle_0 = \exp\{\Xi_1 + \Xi_2 + \dots\}. \tag{14}$$

The expression for the free energy becomes

$$F = F_0 - T(\Xi_1 + \Xi_2 + \dots) = F_0 - T(\langle\mathcal{S}\rangle_{\rm con} - 1). \tag{15}$$

Corrections to the free energy can therefore be expressed as the series $\Xi$ up to a desired order.

We are interested in the lowest order correction which depend on the phase difference of the two superconductors, which is fourth order in the coupling Hamiltonian $H_1$:

$$\Xi_4 = \frac{1}{4!}\int_0^\beta \cdots \int_0^\beta d\tau_1\cdots d\tau_4\,\langle \hat{T}_\tau \hat{H}_1(\tau_1)\hat{H}_1(\tau_2)\hat{H}_1(\tau_3)\hat{H}_1(\tau_4)\rangle, \tag{16}$$

where we define the coupling Hamiltonian as

$$\hat{H}_1 = \sum_\sigma \int dy\left[\sqrt{\lambda_l(y)}\hat{\psi}^\dagger_\sigma(0,y)\hat{\Psi}_\sigma(0,y) + \sqrt{\lambda_r(y)}\hat{\psi}^\dagger_\sigma(W,y)\hat{\Psi}_\sigma(W,y) + \text{H.c.}\right], \tag{17}$$

where the sum is over spin. The coupling is assumed to be on the form:

$$\lambda_{l,r}(y) = |\lambda_{l,r}|e^{2\pi i\varphi_{l,r}(y)}, \tag{18}$$

$$\varphi_{l,r}(y) = \varphi_{l,r}(0) \pm \frac{yB_z(W+W_{SC})}{2\Phi_0}, \tag{19}$$

where $\varphi_{l,r}(y)$ is the phase of the superconductors at $(0,y)$ and $(W,y)$ respectively, $W$ is the width of the junction, and $W_{SC}$ is the width of the superconductors. A gauge has her been chosen such that the vector potential is in the y-direction and vanishes along the center of the junction.

The diagrams of $\Xi_4$ which depends on the phases of both superconductors are

$$\begin{aligned}\Xi_4 = |\lambda_l\lambda_r|\sum_{\sigma_{1..4}}\int dy_{1..4}\int_0^\beta d\tau_{1..4}\\
\times\Big[e^{\frac{i}{2}\Delta\varphi(y_1,y_2,y_3,y_4)}\langle\hat{T}_\tau\hat{\psi}^\dagger_{\sigma_1}(0,y_1;\tau_1)\hat{\Psi}_{\sigma_1}(0,y_1;\tau_1)\hat{\psi}^\dagger_{\sigma_2}(0,y_2;\tau_2)\hat{\Psi}_{\sigma_2}(0,y_2;\tau_2)\\
\times\hat{\Psi}^\dagger_{\sigma_3}(W,y_3;\tau_3)\hat{\psi}_{\sigma_3}(W,y_3;\tau_3)\hat{\Psi}^\dagger_{\sigma_4}(W,y_4;\tau_4)\hat{\psi}_{\sigma_4}(W,y_4;\tau_4)\rangle\\
+e^{-\frac{i}{2}\Delta\varphi(y_1,y_2,y_3,y_4)}\langle\hat{T}_\tau\hat{\psi}^\dagger_{\sigma_1}(W,y_1;\tau_1)\hat{\Psi}_{\sigma_1}(W,y_1;\tau_1)\hat{\psi}^\dagger_{\sigma_2}(W,y_2;\tau_2)\hat{\Psi}_{\sigma_2}(W,y_2;\tau_2)\\
\times\hat{\Psi}^\dagger_{\sigma_3}(0,y_3;\tau_3)\hat{\psi}_{\sigma_3}(0,y_3;\tau_3)\hat{\Psi}^\dagger_{\sigma_4}(0,y_4;\tau_4)\hat{\psi}_{\sigma_4}(0,y_4;\tau_4)\rangle.\Big]\end{aligned} \tag{20}$$

where $\Delta\varphi(y_1,y_2,y_3,y_4) = \frac{1}{2}\left(\varphi_l(y_1)+\varphi_l(y_2)-\varphi_r(y_3)-\varphi_r(y_4)\right)$. We here note that the number of permutations of $H_1(\tau_{1...4})$ cancels with the factor $1/4!$ from before. We now use Wick's theorem to separate these into single particle Greens functions,

$$\begin{aligned}\Xi_4 = -|\lambda_l\lambda_r|\sum_{\sigma_{1..4}}\int dy_{1..4}\int_0^\beta d\tau_{1..4}\\
\times\Big[e^{\frac{i}{2}\Delta\varphi(y_1,y_2,y_3,y_4)}\langle\hat{T}_\tau\hat{\Psi}_{\sigma_1}(0,y_1;\tau_1)\hat{\Psi}_{\sigma_2}(0,y_2;\tau_2)\rangle\langle\hat{T}_\tau\hat{\Psi}^\dagger_{\sigma_3}(W,y_3;\tau_3)\hat{\Psi}^\dagger_{\sigma_4}(W,y_4;\tau_4)\rangle\\
\times\langle\hat{T}_\tau\hat{\psi}_{\sigma_3}(W,y_3;\tau_3)\hat{\psi}^\dagger_{\sigma_1}(0,y_1;\tau_1)\rangle\langle\hat{T}_\tau\hat{\psi}_{\sigma_4}(W,y_4;\tau_4)\hat{\psi}^\dagger_{\sigma_2}(0,y_2;\tau_2)\rangle\\
+e^{-\frac{i}{2}\Delta\varphi(y_1,y_2,y_3,y_4)}\langle\hat{T}_\tau\hat{\Psi}_{\sigma_1}(W,y_1;\tau_1)\hat{\Psi}_{\sigma_2}(W,y_2;\tau_2)\rangle\langle\hat{T}_\tau\hat{\Psi}^\dagger_{\sigma_3}(0,y_3;\tau_3)\hat{\Psi}^\dagger_{\sigma_4}(0,y_4;\tau_4)\rangle\\
\times\langle\hat{T}_\tau\hat{\psi}_{\sigma_3}(0,y_3;\tau_3)\hat{\psi}^\dagger_{\sigma_1}(W,y_1;\tau_1)\rangle\langle\hat{T}_\tau\hat{\psi}_{\sigma_4}(0,y_4;\tau_4)\hat{\psi}^\dagger_{\sigma_2}(W,y_2;\tau_2)\rangle\Big].\end{aligned} \tag{21}$$

We assume that in the normal material, only electron-electron Green functions are non-zero. We define

$$-\langle \hat{T}_\tau \hat{\Psi}_{\sigma_1}(x_1,y_1;\tau_1)\hat{\Psi}_{\sigma_2}(x_2,y_2;\tau_2)\rangle = T\sum_k e^{-i\omega_k(\tau_1-\tau_2)}\mathcal{G}^{\rm sc}_{eh}(x_1,y_1,\sigma_1;x_2,y_2,\sigma_2;i\omega_k), \tag{22}$$

$$\langle \hat{T}_\tau \hat{\psi}_{\sigma_1}(x_1,y_1;\tau_1)\hat{\psi}_{\sigma_2}(x_2,y_2;\tau_2)\rangle = T\sum_k e^{-i\omega_k(\tau_1-\tau_2)}\mathcal{G}(x_1,y_1,\sigma_1;x_2,y_2,\sigma_2;i\omega_k), \tag{23}$$

where the sum is over the fermionic Matsubara frequencies, $\omega_k$. This gives

$$\begin{aligned}\Xi_4 = |\lambda_l\lambda_r|T^4 \sum_{\substack{\sigma_{1..4}\\k_{1..4}}}\int dy_{1..4}\int_0^\beta d\tau_{1..4}\Big[ &- e^{\frac{i}{2}\Delta\varphi(y_1,y_2,y_3,y_4)}e^{-i\omega_{k_1}(\tau_1-\tau_2)}\mathcal{G}^{\rm sc}_{eh}(0,y_1,\sigma_1;0,y_2,\sigma_2;i\omega_{k_1})\\
&\times e^{-i\omega_{k_2}(\tau_3-\tau_4)}\mathcal{G}^{\rm sc}_{he}(W,y_3,\sigma_3;W,y_4,\sigma_4;i\omega_{k_2})\\
&\times e^{-i\omega_{k_3}(\tau_3-\tau_1)}\mathcal{G}(W,y_3,\sigma_3;0,y_1,\sigma_1;i\omega_{k_3})\\
&\times e^{-i\omega_{k_4}(\tau_4-\tau_2)}\mathcal{G}(W,y_4,\sigma_4;0,y_2,\sigma_2;i\omega_{k_4})\\
&- e^{-\frac{i}{2}\Delta\varphi(y_1,y_2,y_3,y_4)}e^{-i\omega_{k_1}(\tau_1-\tau_2)}\mathcal{G}^{\rm sc}_{eh}(W,y_1,\sigma_1;W,y_2,\sigma_2;i\omega_{k_1})\\
&\times e^{-i\omega_{k_2}(\tau_3-\tau_4)}\mathcal{G}^{\rm sc}_{he}(0,y_3,\sigma_3;0,y_4,\sigma_4;i\omega_{k_2})\\
&\times e^{-i\omega_{k_3}(\tau_3-\tau_1)}\mathcal{G}(0,y_3,\sigma_3;W,y_1,\sigma_1;i\omega_{k_3})\\
&\times e^{-i\omega_{k_4}(\tau_4-\tau_2)}\mathcal{G}(0,y_4,\sigma_4;W,y_2,\sigma_2;i\omega_{k_4})\Big]\end{aligned} \tag{24}$$

Now we assume

$$\mathcal{G}^{\rm sc}_{eh}(0,y_1,\sigma_1;0,y_2,\sigma_2;i\omega_k) = \sigma_1\delta(y_1-y_2)\delta_{\sigma_2,\bar{\sigma}_1} \tag{25}$$

$$\mathcal{G}^{\rm sc}_{eh}(W,y_1,\sigma_1;W,y_2,\sigma_2;i\omega_k) = \sigma_1\delta(y_1-y_2)\delta_{\sigma_2,\bar{\sigma}_1} \tag{26}$$

$$\mathcal{G}^{\rm sc}_{he}(0,y_1,\sigma_1;0,y_2,\sigma_2;i\omega_k) = -\sigma_1\delta(y_1-y_2)\delta_{\sigma_2,\bar{\sigma}_1} \tag{27}$$

$$\mathcal{G}^{\rm sc}_{he}(W,y_1,\sigma_1;W,y_2,\sigma_2;i\omega_k) = -\sigma_1\delta(y_1-y_2)\delta_{\sigma_2,\bar{\sigma}_1}, \tag{28}$$

Inserting the assumptions above and performing the integrals over imaginary times, $\tau_{1...4}$, we get

$$\begin{aligned}\Xi_4 = &-|\lambda_l\lambda_r|\sum_{\substack{\sigma_{1..4}\\k_{1..4}}}\int dy_{1..4}\,\delta_{\omega_{k_1},\omega_{k_3}}\delta_{\omega_{k_1},-\omega_{k_4}}\delta_{\omega_{k_2},-\omega_{k_3}}\delta_{\omega_{k_2},\omega_{k_4}}\\
&\times\Big[e^{\frac{i}{2}\Delta\varphi(y_1,y_2,y_3,y_4)}\delta(y_1-y_2)\delta_{\sigma_2,\bar{\sigma}_1}\sigma_1\delta(y_3-y_4)\delta_{\sigma_4,\bar{\sigma}_3}\sigma_3\\
&\qquad\times\mathcal{G}(W,y_3,\sigma_3;0,y_1,\sigma_1;i\omega_{k_3})\mathcal{G}(W,y_4,\sigma_4;0,y_2,\sigma_2;i\omega_{k_4})\\
&\quad+e^{\frac{i}{2}\Delta\varphi(y_1,y_2,y_3,y_4)}\delta(y_1-y_2)\delta_{\sigma_2,\bar{\sigma}_1}\sigma_1\delta(y_3-y_4)\delta_{\sigma_4,\bar{\sigma}_3}\sigma_3\\
&\qquad\times\mathcal{G}(0,y_3,\sigma_3;W,y_1,\sigma_1;i\omega_{k_3})\mathcal{G}(0,y_4,\sigma_4;W,y_2,\sigma_2;i\omega_{k_4})\Big]\end{aligned} \tag{29}$$

We can now integrate over two y-coordinates and do three of the Matsubara frequency sums,

$$\begin{aligned}\Xi_4 = |\lambda_l\lambda_r|\sum_{\sigma,\sigma',k}\sigma\sigma'\int dy\,dy'\big\{&e^{i\Delta\varphi(y,y')}\mathcal{G}(W,y',\sigma';0,y,\sigma;i\omega_k)\mathcal{G}(W,y',\bar{\sigma}';0,y,\bar{\sigma};-i\omega_k)\\
&+e^{-i\Delta\varphi(y,y')}\mathcal{G}(0,y',\sigma';W,y,\sigma;i\omega_k)\mathcal{G}(0,y',\bar{\sigma}';W,y,\bar{\sigma};-i\omega_k)\big\},\end{aligned} \tag{30}$$

where $\Delta\varphi(y,y') = \Delta\varphi(y,y,y',y') = \varphi_l(y)-\varphi_r(y')$. We are free to change the order of summation, $\omega_k\to-\omega_k$ and relabel $y\to y'$ and $\sigma\to\sigma'$ in the second term. Additionally we use the relation,

$$\mathcal{G}(W,y',\sigma';0,y,\sigma;i\omega_k) = \mathcal{G}(0,y,\sigma';W,y',\sigma;-i\omega_k)^*, \tag{31}$$

to get

$$\begin{aligned}\Xi_4 &= |\lambda_l\lambda_r| \sum_{\sigma,\sigma',k} \sigma\sigma' \int dy\, dy' \{ e^{i\Delta\varphi(y,y')} \mathcal{G}(W,y',\sigma';0,y,\sigma;i\omega_k)\mathcal{G}(W,y',\bar{\sigma}';0,y,\bar{\sigma};-i\omega_k) \\ &\qquad + e^{-i\Delta\varphi(y,y')} \mathcal{G}(W,y',\sigma';0,y,\sigma;i\omega_k)^* \mathcal{G}(W,y',\bar{\sigma}';0,y,\bar{\sigma};-i\omega_k)^* \} \\ &= 2|\lambda_l\lambda_r| \sum_{\sigma,\sigma',k} \sigma\sigma' \int dy\, dy' \,\mathrm{Re}\Big\{ e^{i\Delta\varphi(y,y')} \mathcal{G}_{\sigma'\sigma}(W,y';0,y;i\omega_k)\mathcal{G}_{\bar{\sigma}'\bar{\sigma}}(W,y';0,y;-i\omega_k) \Big\},\end{aligned} \tag{32}$$

where we now write the spin labels as subscript indices.

We define the matrix

$$\bar{\mathcal{G}}(x',y';x,y;i\omega_k) = \begin{pmatrix} \mathcal{G}_{\uparrow\uparrow}(x',y';x,y;i\omega_k) & \mathcal{G}_{\uparrow\downarrow}(x',y';x,y;i\omega_k) \\ \mathcal{G}_{\downarrow\uparrow}(x',y';x,y;i\omega_k) & \mathcal{G}_{\downarrow\downarrow}(x',y';x,y;i\omega_k) \end{pmatrix}, \tag{33}$$

which allows us to write

$$\Xi_4 = 2|\lambda_l\lambda_r| \int dy\, dy' \,\mathrm{Re}\Big\{ e^{i\Delta\varphi(y,y')} \sum_k \mathrm{Tr}\big[\bar{\mathcal{G}}(W,y';0,y;i\omega_k)\sigma_y\bar{\mathcal{G}}(W,y';0,y;-i\omega_k)^T\sigma_y\big] \Big\}, \tag{34}$$

The correction to the free energy then becomes:

$$F_4 = -2|\lambda_l\lambda_r| \int dy\, dy' \,\mathrm{Re}\Big\{ e^{i\Delta\varphi(y,y')}\, T \sum_k \mathrm{Tr}\big[\bar{\mathcal{G}}(W,y';0,y;i\omega_k)\sigma_y\bar{\mathcal{G}}(W,y';0,y;-i\omega_k)^T\sigma_y\big] \Big\}. \tag{35}$$

We here make the identification of the induced cooper pair propagator from the supplementary of Ref. [**?** ], describing the propagation from point $(0,y)$ to $(x',y')$ of a induced Cooper pair:

$$C(y',y,x') = T\sum_k \mathrm{Tr}\big[\bar{\mathcal{G}}(x',y';0,y;i\omega_k)\sigma_y\bar{\mathcal{G}}(x',y';0,y;-i\omega_k)^T\sigma_y\big], \tag{36}$$

The sum over Matsubara frequencies can be written as a integral around poles of the complex function $\frac{1}{2}+\frac{1}{2}\tanh(z/2T)$. Assuming zero temperature we get

$$\begin{aligned} C(y',y,x') &= \frac{1}{2\pi i}\left[\int_{-\infty+i0^+}^{\infty+i0^+} dz + \int_{\infty-i0^+}^{-\infty-i0^+} dz\right]\left[\frac{1}{2}+\frac{1}{2}\tanh\Big(\frac{z}{2T}\Big)\right] \\ &\qquad \times \mathrm{Tr}\big[\bar{\mathcal{G}}(x',y';0,y;z)\sigma_y\bar{\mathcal{G}}(x',y';0,y;-z)^T\sigma_y\big] \\ &= \frac{1}{2\pi i}\int_0^\infty d\omega\, \mathrm{Tr}\Big[\bar{G}^R(x',y';0,y;\omega)\sigma_y\bar{G}^A(x',y';0,y;-\omega)^T\sigma_y \\ &\qquad - \bar{G}^A(x',y';0,y;\omega)\sigma_y\bar{G}^R(x',y';0,y;-\omega)^T\sigma_y\Big]. \end{aligned} \tag{37}$$

Where $\bar{G}^{A,R}$ are the advanced and retarded Green functions. In terms of the two spin eigenstates, $|\lambda_k\rangle$, these Green functions can be written as:

$$\bar{G}^{R,A}(x',y';0,y;\omega) = \frac{1}{(2\pi)^2}\int d\mathbf{k}\, e^{i\mathbf{k}\cdot\mathbf{r}} \sum_{\lambda_\mathbf{k}} \frac{|\lambda_\mathbf{k}\rangle\langle\lambda_\mathbf{k}|}{\omega-\epsilon_{\mathbf{k}\lambda}\pm i\eta}, \tag{38}$$

where $\mathbf{r} = \{x', y'-y\}$ and $\eta$ is an infinitesimally small number. This gives

$$\begin{aligned} C(\mathbf{r}) &= \frac{1}{2\pi i}\frac{1}{(2\pi)^4}\int_0^\infty d\omega \int d\mathbf{k}\, d\mathbf{k}'\, \mathrm{Tr}\Bigg[\sum_{\lambda_\mathbf{k},\lambda_{\mathbf{k}'}} e^{i\mathbf{k}\cdot\mathbf{r}}e^{i\mathbf{k}'\cdot\mathbf{r}} \\ &\times \left(\frac{|\lambda_\mathbf{k}\rangle\langle\lambda_\mathbf{k}|}{\omega-\epsilon_{\mathbf{k}\lambda}+i0}\sigma_y\frac{|\lambda_{\mathbf{k}'}\rangle\langle\lambda_{\mathbf{k}'}|^T}{-\omega-\epsilon_{\mathbf{k}'\lambda}-i0}\sigma_y - \frac{|\lambda_\mathbf{k}\rangle\langle\lambda_\mathbf{k}|}{\omega-\epsilon_{\mathbf{k}\lambda}-i0}\sigma_y\frac{|\lambda_{\mathbf{k}'}\rangle\langle\lambda_{\mathbf{k}'}|^T}{-\omega-\epsilon_{\mathbf{k}'\lambda}+i0}\sigma_y\right)\Bigg], \end{aligned} \tag{39}$$

We now use that

$$\frac{1}{\omega-\epsilon_{\mathbf{k}\lambda}+i0}\frac{1}{-\omega-\epsilon_{\mathbf{k}'\lambda}-i0}-\frac{1}{\omega-\epsilon_{\mathbf{k}\lambda}-i0}\frac{1}{-\omega-\epsilon_{\mathbf{k}'\lambda}+i0}$$
$$=-2\pi i\frac{\delta(\omega-\epsilon_{\mathbf{k}\lambda})}{-\omega-\epsilon_{\mathbf{k}'\lambda}}+2\pi i\frac{\delta(\omega+\epsilon_{\mathbf{k}'\lambda})}{\omega-\epsilon_{\mathbf{k}\lambda}}, \tag{40}$$

to show that

$$\begin{aligned}
C(\mathbf{r}) &= \frac{1}{(2\pi)^4}\int_0^\infty d\omega\int d\mathbf{k}\,d\mathbf{k}' \\
&\quad\times \mathrm{Tr}\left[\sum_{\lambda_\mathbf{k},\lambda_{\mathbf{k}'}} e^{i\mathbf{k}\cdot\mathbf{r}}e^{i\mathbf{k}'\cdot\mathbf{r}}\left(\frac{\delta(\omega+\epsilon_{\mathbf{k}'\lambda})}{\omega-\epsilon_{\mathbf{k}\lambda}}-\frac{\delta(\omega-\epsilon_{\mathbf{k}\lambda})}{-\omega-\epsilon_{\mathbf{k}'\lambda}}\right)|\lambda_\mathbf{k}\rangle\langle\lambda_\mathbf{k}|\,\sigma_y\,|\lambda_{\mathbf{k}'}\rangle\langle\lambda_{\mathbf{k}'}|^T\,\sigma_y\right] \\
&= \frac{1}{(2\pi)^4}\int_0^\infty d\omega\int d\mathbf{k}\,d\mathbf{k}' \\
&\quad\times \mathrm{Tr}\left[\sum_{\lambda_\mathbf{k},\lambda_{\mathbf{k}'}} e^{i\mathbf{k}\cdot\mathbf{r}}e^{i\mathbf{k}'\cdot\mathbf{r}}\left(\frac{\delta(\omega+\epsilon_{\mathbf{k}'\lambda})}{\omega-\epsilon_{\mathbf{k}\lambda}}+\frac{\delta(\omega-\epsilon_{\mathbf{k}\lambda})}{\omega+\epsilon_{\mathbf{k}'\lambda}}\right)|\lambda_\mathbf{k}\rangle\langle\lambda_\mathbf{k}|\,\sigma_y\,|\lambda_{\mathbf{k}'}\rangle\langle\lambda_{\mathbf{k}'}|^T\,\sigma_y\right] \\
&= \frac{1}{(2\pi)^4}\int d\mathbf{k}\,d\mathbf{k}' \\
&\quad\times \mathrm{Tr}\left[\sum_{\lambda_\mathbf{k},\lambda_{\mathbf{k}'}} e^{i\mathbf{k}\cdot\mathbf{r}}e^{i\mathbf{k}'\cdot\mathbf{r}}\left(\frac{\theta(-\epsilon_{\mathbf{k}'\lambda})}{-\epsilon_{\mathbf{k}'\lambda}-\epsilon_{\mathbf{k}\lambda}}+\frac{\theta(\epsilon_{\mathbf{k}\lambda})}{\epsilon_{\mathbf{k}\lambda}+\epsilon_{\mathbf{k}'\lambda}}\right)|\lambda_\mathbf{k}\rangle\langle\lambda_\mathbf{k}|\,\sigma_y\,|\lambda_{\mathbf{k}'}\rangle\langle\lambda_{\mathbf{k}'}|^T\,\sigma_y\right],
\end{aligned} \tag{41}$$

where $\theta(x)$ is the Heaviside step function, which comes from the fact that only positive $\omega$ are considered in the integral. Instead of the step function we introduce two energies $\epsilon$ and $\epsilon'$ which picks out the same parts of the integral,

$$\begin{aligned}
C(\mathbf{r}) &= \frac{1}{(2\pi)^4}\int d\mathbf{k}\,d\mathbf{k}'\sum_{\lambda_\mathbf{k},\lambda_{\mathbf{k}'}} e^{i\mathbf{k}\cdot\mathbf{r}}e^{i\mathbf{k}'\cdot\mathbf{r}}\,|\lambda_\mathbf{k}\rangle\langle\lambda_\mathbf{k}|\,\sigma_y\,|\lambda_{\mathbf{k}'}\rangle\langle\lambda_{\mathbf{k}'}|^T\,\sigma_y \\
&\quad\times \mathrm{Tr}\left[\int d\epsilon\int_{-\infty}^0 d\epsilon'\frac{\delta(\epsilon'-\epsilon_{\mathbf{k}'\lambda})\delta(\epsilon-\epsilon_{\mathbf{k}\lambda})}{-\epsilon'-\epsilon}+\int_0^\infty d\epsilon\int d\epsilon'\frac{\delta(\epsilon'-\epsilon_{\mathbf{k}'\lambda})\delta(\epsilon-\epsilon_{\mathbf{k}\lambda})}{\epsilon'+\epsilon}\right] \\
&= \frac{1}{(2\pi)^4}\int d\mathbf{k}\,d\mathbf{k}'\sum_{\lambda_\mathbf{k},\lambda_{\mathbf{k}'}} e^{i\mathbf{k}\cdot\mathbf{r}}e^{i\mathbf{k}'\cdot\mathbf{r}}\,|\lambda_\mathbf{k}\rangle\langle\lambda_\mathbf{k}|\,\sigma_y\,|\lambda_{\mathbf{k}'}\rangle\langle\lambda_{\mathbf{k}'}|^T\,\sigma_y \\
&\quad\times \mathrm{Tr}\left[\int_0^\infty d\epsilon\int d\epsilon'\frac{\delta(\epsilon'-\epsilon_{\mathbf{k}'\lambda})\delta(\epsilon-\epsilon_{\mathbf{k}\lambda})}{\epsilon'+\epsilon}-\int d\epsilon\int_{-\infty}^0 d\epsilon'\frac{\delta(\epsilon'-\epsilon_{\mathbf{k}'\lambda})\delta(\epsilon-\epsilon_{\mathbf{k}\lambda})}{\epsilon'+\epsilon}\right].
\end{aligned} \tag{42}$$

When $\epsilon > 0$ and $\epsilon' < 0$ the two integrals are equal, and therefore cancel,

$$\begin{aligned}
C(\mathbf{r}) &= \frac{1}{(2\pi)^4}\int d\mathbf{k}\,d\mathbf{k}'\sum_{\lambda_\mathbf{k},\lambda_{\mathbf{k}'}} e^{i\mathbf{k}\cdot\mathbf{r}}e^{i\mathbf{k}'\cdot\mathbf{r}}\,|\lambda_\mathbf{k}\rangle\langle\lambda_\mathbf{k}|\,\sigma_y\,|\lambda_{\mathbf{k}'}\rangle\langle\lambda_{\mathbf{k}'}|^T\,\sigma_y \\
&\quad\times \mathrm{Tr}\left[\int_0^\infty d\epsilon\int_0^\infty d\epsilon'\frac{\delta(\epsilon'-\epsilon_{\mathbf{k}'\lambda})\delta(\epsilon-\epsilon_{\mathbf{k}\lambda})}{\epsilon'+\epsilon}-\int_{-\infty}^0 d\epsilon\int_{-\infty}^0 d\epsilon'\frac{\delta(\epsilon'-\epsilon_{\mathbf{k}'\lambda})\delta(\epsilon-\epsilon_{\mathbf{k}\lambda})}{\epsilon'+\epsilon}\right] \\
&= \frac{1}{(2\pi)^4}\int d\mathbf{k}\,d\mathbf{k}'\sum_{\lambda_\mathbf{k},\lambda_{\mathbf{k}'}} e^{i\mathbf{k}\cdot\mathbf{r}}e^{i\mathbf{k}'\cdot\mathbf{r}}\,|\lambda_\mathbf{k}\rangle\langle\lambda_\mathbf{k}|\,\sigma_y\,|\lambda_{\mathbf{k}'}\rangle\langle\lambda_{\mathbf{k}'}|^T\,\sigma_y \\
&\quad\times \mathrm{Tr}\left[\int_0^\infty d\epsilon\int_0^\infty d\epsilon'\frac{\delta(\epsilon'-\epsilon_{\mathbf{k}'\lambda})\delta(\epsilon-\epsilon_{\mathbf{k}\lambda})}{\epsilon'+\epsilon}+\int_0^\infty d\epsilon\int_0^\infty d\epsilon'\frac{\delta(-\epsilon'-\epsilon_{\mathbf{k}'\lambda})\delta(-\epsilon-\epsilon_{\mathbf{k}\lambda})}{\epsilon'+\epsilon}\right].
\end{aligned} \tag{43}$$

We now define a spectral function

$$\bar{g}(\mathbf{r},\epsilon)=\frac{1}{(2\pi)^2}\int d\mathbf{k}\sum_{\lambda_\mathbf{k}} e^{i\mathbf{k}\cdot\mathbf{r}}\delta(\epsilon-\epsilon_{\mathbf{k}\lambda})\,|\lambda_\mathbf{k}\rangle\langle\lambda_\mathbf{k}|, \tag{44}$$

which gives us the expression

$$C(\mathbf{r}) = \int_0^\infty d\epsilon \int_0^\infty d\epsilon' \frac{\mathrm{Tr}\big[\bar{g}(\mathbf{r},\epsilon)\sigma_y \bar{g}(\mathbf{r},\epsilon')^T\sigma_y + \bar{g}(\mathbf{r},-\epsilon)\sigma_y \bar{g}(\mathbf{r},-\epsilon')^T\sigma_y\big]}{\epsilon+\epsilon'}, \tag{45}$$

## II. SEMI-CLASSICAL APPROXIMATION OF THE COOPER PAIR PROPAGATOR

We now consider a specific Hamiltonian with some assumptions. The Hamiltonian we consider is a $2 \times 2$ linear Hamiltonian with some combination of effective fields (e.g. Zeeman and spin orbit interaction),

$$H_{\mathbf{k}} = v_F(k-k_F) + \vec{\beta}(\hat{k})\cdot\vec{\sigma}, \tag{46}$$

where $v_F$ is the Fermi velocity, $k_F$ is the Fermi momentum, $\vec{\sigma}$ is a vector of the three Pauli spin matrices, and $\beta$ is the effective field which can depend on the direction of the momentum $\hat{k} = \mathbf{k}/|\mathbf{k}|$. In terms of a projection operator, projecting to the spin eigenstates mentioned above, we write,

$$H_{\mathbf{k}} = \sum_{\lambda_{\mathbf{k}}} \epsilon_{\lambda_{\mathbf{k}}} P^{\lambda_{\mathbf{k}}}, \tag{47}$$

$$\epsilon_{\lambda_{\mathbf{k}}} = v_F(k-k_f) + \lambda|\vec{\beta}|, \tag{48}$$

$$P^{\lambda_{\mathbf{k}}} = (\mathbb{1} + \lambda\hat{\beta}(\hat{k})\cdot\vec{\sigma})/2. \tag{49}$$

Where $\lambda = \pm 1$ corresponds to which of the two eigenstates, $|\lambda_{\mathbf{k}}\rangle$, we are talking about. This projector can be inserted into the expression for the spectral function above (44):

$$\bar{g}(\mathbf{r},\epsilon) = \frac{1}{(2\pi)^2}\sum_{\lambda_{\mathbf{k}}}\int d\mathbf{k}\, e^{i\mathbf{k}\cdot\mathbf{r}}\delta(\epsilon-\epsilon_{\mathbf{k}\lambda})P^{\lambda_{\mathbf{k}}}, \tag{50}$$

Inserting the expression above and writing the integral on polar form we get

$$\begin{aligned}\bar{g}(\mathbf{r},\epsilon) &= \frac{1}{(2\pi)^2}\sum_{\lambda_{\mathbf{k}}}\int_0^{2\pi}\frac{d\theta}{v_F}\left(\frac{\epsilon-\lambda|\vec{\beta}(\hat{k})|}{v_F}+k_F\right)e^{i\left(\frac{\epsilon-\lambda|\vec{\beta}(\hat{k})|}{v_F}+k_F\right)r\cos\theta}P^{\lambda_{\mathbf{k}}}\\ &\approx \frac{k_F}{(2\pi)^2 v_F}\sum_{\lambda_{\mathbf{k}}}\int_0^{2\pi} d\theta e^{i\left(\frac{\epsilon-\lambda|\vec{\beta}(\hat{k})|}{v_F}+k_F\right)r\cos\theta}P^{\lambda_{\mathbf{k}}}\end{aligned} \tag{51}$$

in the last step have assumed that $\frac{\epsilon-\lambda|\vec{\beta}(\hat{k})|}{v_F} \ll k_F$. Implying that the everything happens close to the Fermi-energy.

To solve this integral we need some information about the projector and hence the effective field. Here we define the total effective field as made up of two in plane effective fields with some general winding, $m$ and $n$. With winding we mean that when the momentum vector rotates once the effective fields rotates $m$ and $n$ times respectively. Examples of effective fields are the Zeeman field, which does not wind, and Rashba and Dresselhaus spin orbit coupling, which winds $m = 1$ and $m = -1$ times respectively.

$$\vec{\beta}(\theta) = (\alpha\cos(m\theta+\phi_\alpha)+\beta\cos(n\theta+\phi_\beta), \alpha\sin(m\theta+\phi_\alpha)+\beta\sin(n\theta+\phi_\beta), 0) \tag{52}$$

Where $\alpha$ and $\beta$ are the amplitudes of the two effective fields, and $\phi_{\alpha,\beta}$ are arbitrary phases, and $\theta$ is the angle of $\mathbf{k}$.

The projector then becomes

$$P^{\lambda_{\mathbf{k}}} = \begin{pmatrix} \frac{1}{2} & \frac{\lambda(\beta_x(\hat{k})-i\beta_y(\hat{k}))}{2|\vec{\beta}(\hat{k})|} \\ \frac{\lambda(\beta_x(\hat{k})+i\beta_y(\hat{k}))}{2|\vec{\beta}(\hat{k})|} & \frac{1}{2}\end{pmatrix} \tag{53}$$

$$\frac{\lambda(\beta_x(\hat{k})\pm i\beta_y(\hat{k}))}{2|\vec{\beta}(\hat{k})|} = \frac{\lambda\left(\alpha\cos(m\theta+\phi_\alpha)+\beta\cos(n\theta+\phi_\beta)\pm i\left(\alpha\sin(m\theta+\phi_\alpha)+\beta\sin(n\theta+\phi_\beta)\right)\right)}{2\sqrt{\left(\alpha\cos(m\theta+\phi_\alpha)+\beta\cos(n\theta+\phi_\beta)\right)^2+\left(\alpha\sin(m\theta+\phi_\alpha)+\beta\sin(n\theta+\phi_\beta)\right)^2}} \tag{54}$$

The numerator can obviously be written as a sum of terms on the form $Ce^{\pm i(l\theta+\phi)}$ where $C$ and $\phi$ are constant in $\theta$. If we take the Taylor series of $1/|\beta(\hat{k})|$ around e.g. $\alpha = 0$, every term here can also be written on the form $Ce^{\pm i(l\theta+\phi)}$.

This means that the whole projector can be written as an infinite series of terms on the same form. The general integral we have to solve is therefore

$$\int_0^{2\pi} d\theta e^{i\tilde{k}_F(\theta) r\cos\theta} e^{\pm il\theta}, \tag{55}$$

where $\tilde{k}_F(\theta) = \frac{-\lambda|\vec{\beta}(\theta)|}{v_F} + k_F$ and we have excluded constant factors. What we will see is that the result of these integrals can be re-summed to the propagator, evaluated in two directions of $\mathbf{k}$. To solve this integral we use the so called Jacobi-Anger expansion

$$e^{iz\cos(\theta)} = \sum_{n=-\infty}^{\infty} i^n J_n(z) e^{in\theta}, \tag{56}$$

where $J_n(z)$ are Bessel functions. The integral then becomes

$$\int_0^{2\pi} d\theta e^{i\tilde{k}_F(\theta) r\cos\theta} e^{\pm il\theta} = \int_0^{2\pi} d\theta \sum_n i^n J_n\left(\tilde{k}_F(\theta) r\right) e^{in\theta} e^{\pm il\theta} \tag{57}$$

next we use the assumption that $k_F r \gg 1$ to employ the big parameter limit of the Bessel functions $J_n(z) \overset{z\gg 1}{\approx} \sqrt{\frac{2}{\pi z}}\cos(-z + \frac{\pi}{4} + \frac{n\pi}{2})$

$$\begin{aligned}
\int_0^{2\pi} d\theta e^{i\tilde{k}_F(\theta) r\cos\theta} e^{\pm il\theta} &\approx \int_0^{2\pi} d\theta \sum_n i^n \sqrt{\frac{2}{\pi k_F r}} \cos\left(-\tilde{k}_F(\theta) r + \frac{\pi}{4} + \frac{n\pi}{2}\right) e^{in\theta} e^{\pm il\theta} \\
&= \frac{1}{2}\int_0^{2\pi} d\theta \sum_n \sqrt{\frac{2}{\pi k_F r}} \\
&\quad \times \left[e^{i\left(-\tilde{k}_F(\theta) r + \frac{\pi}{4}\right)} e^{in(\theta+\pi)} + e^{-i\left(-\tilde{k}_F(\theta) r + \frac{\pi}{4}\right)} e^{in\theta}\right] e^{\pm il\theta} \\
&= \frac{1}{2}\int_0^{2\pi} d\theta \sqrt{\frac{2}{\pi k_F r}} \\
&\quad \times \left[e^{i\left(-\tilde{k}_F(\theta) r + \frac{\pi}{4}\right)} 2\pi\delta(\theta+\pi) + e^{-i\left(-\tilde{k}_F(\theta) r + \frac{\pi}{4}\right)} 2\pi\delta(\theta)\right] e^{\pm il\theta}
\end{aligned} \tag{58}$$

where in the last step we have carried out the sum over $n$ using the Fourier series representation of the Dirac delta function:

$$\begin{aligned}
\delta(x) &= \frac{1}{2\pi} + \frac{1}{\pi}\sum_{n=1}^{\infty}\cos(nx) \\
&= \frac{1}{2\pi}\sum_n e^{inx}.
\end{aligned} \tag{59}$$

We use the delta functions to solve the integral,

$$\int_0^{2\pi} d\theta e^{i\tilde{k}_F(\theta) r\cos\theta} e^{\pm il\theta} \approx \sqrt{\frac{2\pi}{k_F r}} \left[e^{i\left(-\tilde{k}_F(\pi) r + \frac{\pi}{4}\right)} e^{\pm il\pi} + e^{i\left(\tilde{k}_F(0) r - \frac{\pi}{4}\right)} e^{\pm il0}\right]. \tag{60}$$

As mentioned, since the integral of any term in the series expansion of the propagator amounts to evaluating in $\theta = \pi$ and $\theta = 0$, the series can be re-summed to get the projector, now evaluated in the two directions. The spectral function $g(\epsilon, \vec{r})$ becomes:

$$\begin{aligned}
g(\epsilon,\vec{r}) &\approx \frac{k_F}{(2\pi)^2 v_F}\sum_\lambda \sqrt{\frac{2\pi}{k_F r}} \left[e^{i\left(\frac{\epsilon-\lambda|\beta^+|}{v_F}+k_F\right) r - i\pi/4} P^{\lambda_+} + e^{-i\left(\frac{\epsilon-\lambda|\beta^-|}{v_F}+k_F\right) r + i\pi/4} P^{\lambda_-}\right] \\
&= \frac{\sqrt{k_F}}{(2\pi)^{3/2} v_F \sqrt{r}} \sum_\lambda \left[e^{i\left(\frac{\epsilon-\lambda|\beta^+|}{v_F}+k_F\right) r - i\pi/4} P^{\lambda_+} + e^{-i\left(\frac{\epsilon-\lambda|\beta^-|}{v_F}+k_F\right) r + i\pi/4} P^{\lambda_-}\right]
\end{aligned} \tag{61}$$

where $P^{\lambda\pm}$ and $\beta^{\pm}$ are the projector, $P^{\lambda_{\mathbf{k}}}$, and the effective field, $\beta(\hat{k})$, respectively evaluated for $\vec{k}$ parallel/anti-parallel to $\vec{r}$ (i.e. $\theta = 0$ and $\theta = \pi$). This can now be inserted into the expression for the cooper pair propagator

$$\begin{aligned}&\int_{-\infty}^{0}\int_{-\infty}^{0} d\epsilon d\epsilon' \frac{\mathrm{Tr}\left\{g(\epsilon,\vec{r})\sigma_y g^T(\epsilon',\vec{r})\sigma_y + g(-\epsilon',\vec{r})\sigma_y g^T(-\epsilon,\vec{r})\sigma_y\right\}}{(\epsilon+\epsilon')} \\ &\approx \frac{k_F}{(2\pi)^3 v_F^2 r}\int_{-\infty}^{0}\int_{-\infty}^{0} d\epsilon d\epsilon' \\ &\quad\times \frac{\mathrm{Tr}\left\{\sum_{\lambda\lambda'}\left[P^{\lambda+}\sigma_y P^{\lambda'_-T}\sigma_y + P^{\lambda'_-}\sigma_y P^{\lambda+T}\sigma_y\right] e^{i(\epsilon-\epsilon')r/v_F} e^{-i(\lambda|\beta^+|-\lambda'|\beta^-|)r/v_F}\right\}}{(\epsilon+\epsilon')}\end{aligned} \tag{62}$$

The $\epsilon$ integrals can now be carried out, using the identity $\iint_{-\infty}^{0} d\epsilon d\epsilon' \frac{e^{\pm i(\epsilon-\epsilon')a}}{\epsilon+\epsilon'} = \frac{\pi}{2a}$,

$$\begin{aligned}&\int_{-\infty}^{0}\int_{-\infty}^{0} d\epsilon d\epsilon' \frac{\mathrm{Tr}\left\{g(\epsilon,\vec{r})\sigma_y g^T(\epsilon',\vec{r})\sigma_y + g(-\epsilon',\vec{r})\sigma_y g^T(-\epsilon,\vec{r})\sigma_y\right\}}{(\epsilon+\epsilon')} \\ &\approx \frac{2k_F}{(4\pi)^2 v_F r^2}\mathrm{Tr}\left\{\sum_{\lambda\lambda'}\left[P^{\lambda+}\sigma_y P^{\lambda_-T}\sigma_y + P^{\lambda'_-}\sigma_y P^{\lambda'_+T}\sigma_y\right]\right\} e^{-i(\lambda|\beta^+|-\lambda'|\beta^-|)r/v_F}\end{aligned} \tag{63}$$

We now use that:

$$P^{\lambda\pm} = \left(\mathbb{1} + \lambda\hat{\beta}^{\pm}\cdot\vec{\sigma}\right)/2 \tag{64}$$

$$\sigma_y P^{\lambda\pm T}\sigma_y = \left(\mathbb{1} - \lambda\hat{\beta}^{\pm}\cdot\vec{\sigma}\right)/2, \tag{65}$$

And that all terms proportional a sigma matrix vanishes under the spin trace, to show that:

$$\begin{aligned}&\mathrm{Tr}\left\{\sum_{\lambda\lambda'}\left[P^{\lambda+}\sigma_y P^{\lambda'_-T}\sigma_y + P^{\lambda'_-}\sigma_y P^{\lambda+T}\sigma_y\right]\right\} \\ &= \mathrm{Tr}\left\{\sum_{\lambda\lambda'}\left(\mathbb{1} - \lambda\lambda'(\hat{\beta}^+\cdot\vec{\sigma})(\hat{\beta}^-\cdot\vec{\sigma})\right)/2\right\}.\end{aligned} \tag{66}$$

We use the identity $(\vec{a}\cdot\vec{\sigma})(\vec{b}\cdot\vec{\sigma}) = (\vec{a}\cdot\vec{b})\mathbb{1} + i(\vec{a}\times\vec{b})\vec{\sigma}$ and again the fact that terms proportional to sigma matrices vanish under the trace to get:

$$\begin{aligned}&\mathrm{Tr}\left\{\sum_{\lambda\lambda'}\left[P^{\lambda+}\sigma_y P^{\lambda'_-T}\sigma_y + P^{\lambda'_-}\sigma_y P^{\lambda+T}\sigma_y\right]\right\} \\ &= \sum_{\lambda\lambda'}\left(1 - \lambda\lambda'(\hat{\beta}^+\cdot\hat{\beta}^-)\right)\end{aligned} \tag{67}$$

This then gives us the expression for the cooper pair propagator

$$\begin{aligned}C(\mathbf{r}) &= \int_{-\infty}^{0}\int_{-\infty}^{0} d\epsilon d\epsilon' \frac{\mathrm{Tr}\left\{g(\epsilon,\vec{r})\sigma_y g^T(\epsilon',\vec{r})\sigma_y + g(-\epsilon',\vec{r})\sigma_y g^T(-\epsilon,\vec{r})\sigma_y\right\}}{(\epsilon+\epsilon')} \\ &\approx \frac{2k_F}{(4\pi)^2 v_F r^2}\sum_{\lambda\lambda'}\left(1 - \lambda\lambda'(\hat{\beta}^+\cdot\hat{\beta}^-)\right) e^{-i(\lambda|\beta^+|-\lambda'|\beta^-|)r/v_F}\end{aligned} \tag{68}$$

## III. SPECIAL CASES OF THE COOPER PAIR PROPAGATOR

Here we discuss some limiting cases of the pair propagator in equation (68). We always look at the case where we have two terms contributing to the effective field. In the case where either is dominating over the other (or in are equal in one of the cases) we can simplify the expression above.

**Large HH-LH splitting**

*Large cubic Rashba SOI, $|\beta_{12}| \ll |\beta_{03}|$*

Given that $|\beta_{12}| \ll |\beta_{03}|$ we get the zeroth order approximation:

$$\vec{\beta}(\hat{k}) \approx -\vec{\beta}(-\hat{k}) \tag{69}$$

By taking this approximation the prefactor, $\Big(1 - \lambda\lambda'(\hat{\beta}^{+} \cdot \hat{\beta}^{-})\Big)$, in the cooper pair propagator is proportional to the dirac delta function, $\delta_{\lambda\lambda'}$. Taking the same approximation in the exponential would mean that it will cancel fully and so here we take the first order correction to this:

$$\begin{aligned} |\vec{\beta}_{\pm}| &\approx |\beta_{03}|\sqrt{1 \pm 2\frac{|\beta_{12}|}{|\beta_{03}|}(\hat{\beta}_{12} \cdot \hat{\beta}_{03})} \\ &\approx |\beta_{03}| \pm |\beta_{12}|(\hat{\beta}_{12} \cdot \hat{\beta}_{03}) \end{aligned} \tag{70}$$

The exponential then becomes:

$$e^{i\lambda(|\beta_{+}|-|\beta_{-}|)r/v_F} = e^{i\lambda(2|\beta_{12}|(\hat{\beta}_{12}\cdot\hat{\beta}_{03}))r/v_F} \tag{71}$$

As we can see, the cooper pair propagator only care about the dot product of the effective fields, and it is therefore clear why the additional $2\theta_k + \pi$ winding in both effective fields compared to the case of the 2DEG are irrelevant.

$$\begin{aligned} \hat{\beta}_{12} \cdot \hat{\beta}_{03} &= \sin(\theta_B + 2\theta_k + \pi)\sin(3\theta_k + \frac{3\pi}{2}) + \cos(\theta_B + 2\theta_k + \pi)\cos(3\theta_k + \frac{3\pi}{2}) \\ &= \sin(\theta_B)\sin(\theta_k + \frac{\pi}{2}) + \cos(\theta_B)\cos(\theta_k + \frac{\pi}{2}) \\ &= \hat{B}_x\hat{k}_y - \hat{B}_y\hat{k}_x \\ &= \Big(\hat{z} \times \hat{B}\Big) \cdot \hat{k} \end{aligned} \tag{72}$$

*Small cubic Rashba SOI, $|\beta_{12}| \gg |\beta_{03}|$*

We do a similar approximation as above, but now the total effective field is approximately even:

$$\vec{\beta}_{+} \approx \vec{\beta}_{-} \tag{73}$$

And so the prefactor, $\Big(1 - \lambda\lambda'(\hat{\beta}^{+} \cdot \hat{\beta}^{-})\Big)$, can be approximated as the dirac delta function, $\delta_{-\lambda\lambda'}$. Here however, the lowest order non trivial term is the zeroth order term:

$$e^{i\lambda(|\beta_{+}|+|\beta_{-}|)r/v_F} \approx e^{2i\lambda|\beta_{12}|r/v_F} \tag{74}$$

**Small Luttinger coupling**

The arguments from the previous section still hold here, the results above still hold with the substitutions $\hat{\beta}_{12}\cdot\hat{\beta}_{03} \rightarrow \hat{\beta}_{30} \cdot \hat{\beta}_{21}$ and $|\beta_{12}| \rightarrow |\beta_{30}|$. The dot product in fact becomes the same as well:

$$\begin{aligned} \hat{\beta}_{30} \cdot \hat{\beta}_{21} &= \sin(3\theta_B)\sin(2\theta_B + \theta_k + \frac{\pi}{2}) + \cos(3\theta_B)\cos(2\theta_B + \theta_k + \frac{\pi}{2}) \\ &= \sin(\theta_B)\cos(\theta_k) - \cos(\theta_B)\sin(\theta_k) \\ &= \Big(\hat{z} \times \hat{B}\Big) \cdot \hat{k} \end{aligned} \tag{75}$$

**Large Rashba amplitude**

The effective field in this case is fully odd in k, $\vec{\beta}_+ = -\vec{\beta}_-$:

$$\vec{\beta}(\theta) = \frac{\alpha k_F}{\Delta}\begin{bmatrix}\frac{k_F^2}{2m_x}\cos(3\theta_k) + \frac{(2\kappa\mu_B|B_\parallel|)^2}{\Delta}\cos(\theta_k + 2\theta_B)\\ \frac{k_F^2}{2m_x}\sin(3\theta_k) + \frac{(2\kappa\mu_B|B_\parallel|)^2}{\Delta}\sin(\theta_k + 2\theta_B)\end{bmatrix} \tag{76}$$

The prefactor in the cooper pair propagator $\left(1 - \lambda\lambda'(\hat{\beta}^+ \cdot \hat{\beta}^-)\right)$ simplifies to the dirac delta function, $2\delta_{\lambda\lambda'}$. The exponential also simplifies, since we now have $\lambda = \lambda'$ and $|\vec{\beta}_+| = |\vec{\beta}_-|$. The terms in the exponential cancels and we are left with:

$$C(\mathbf{r}) = \frac{2K}{r^2}, \tag{77}$$

where $K = \frac{2k_F}{(4\pi)^2 v_F}$.

**Small Rashba amplitude**

The effective field now is fully even in momentum, $\vec{\beta}_+ = \vec{\beta}_-$:

$$\vec{\beta}(\theta) = \frac{-2\kappa\mu_B|B_\parallel|}{\Delta}\begin{bmatrix}\frac{k_F^2}{2m_x}\cos(2\theta_k + \theta_B)\\ + \frac{(2\kappa\mu_B|B_\parallel|)^2}{\Delta}\cos(3\theta_B)\\ \\ \frac{k_F^2}{2m_x}\sin(2\theta_k + \theta_B)\\ + \frac{(2\kappa\mu_B|B_\parallel|)^2}{\Delta}\sin(3\theta_B)\end{bmatrix} \tag{78}$$

In a similar argument as above the prefactor in cooper pair propagator, $\left(1 - \lambda\lambda'(\hat{\beta}^+ \cdot \hat{\beta}^-)\right)$, becomes proportional to the dirac delta function $\delta_{-\lambda\lambda'}$. Instead of the terms in the exponential canceling they now add up to:

$$\begin{aligned} C(\mathbf{r}) &= \sum_\lambda \frac{2K}{r^2} e^{2i\lambda|\beta(\hat{r})|r/v_F}. \\ &= \frac{K}{r^2}\cos(2|\beta(\hat{r})|r/v_F) \end{aligned} \tag{79}$$

where still $K = \frac{2k_F}{(4\pi)^2 v_F}$. In the case where either of the two components of the effective field i dominating, the magnitude of the effective field to zeroth order becomes:

$$|\vec{\beta}| = \begin{cases} \left|\frac{(2\kappa\mu_B|B_\parallel|)^3}{\Delta^2}\right|, & |\vec{\beta}_{12}| \ll |\vec{\beta}_{30}| \\ \left|\frac{2\kappa\mu_B|B_\parallel|k_F^2}{2m_x\Delta}\right|, & |\vec{\beta}_{12}| \gg |\vec{\beta}_{30}| \end{cases} \tag{80}$$

For the special case of the magnitudes of the two components being equal, $|\beta_{12}| = |\beta_{30}|$, we have:

$$\begin{aligned} |\beta| &= |\beta_{12/30}|\sqrt{(\cos(2\theta_k + \pi + \theta_B) + \cos(3\theta_B))^2 + (\sin(2\theta_k + \pi + \theta_B) + \sin(3\theta_B))^2} \\ &= 2|\beta_{12/30}|\,|\cos(\theta_B)\cos(\theta_k) + \sin(\theta_B)\sin(\theta_k)| \\ &= 2|\beta_{12/30}|\left|\hat{B}\cdot\hat{k}\right| \end{aligned} \tag{81}$$

## IV. ANALYTIC EXPRESSION FOR CRITICAL CURRENT

For the second case, with the dot-product, no approximation of the integrand is needed:

$$\begin{aligned}
I_{\mathrm{d}}(\vec{\beta}) &= \iint dy\, dy_1\, \frac{\cos(\vec{\beta}\cdot\vec{r})}{r^2} \\
&= \Bigg\{ -i\cosh((\beta_x - i\beta_y)W)\Big[D^*\mathrm{Ci}(\beta_x D^*) - D\mathrm{Ci}(-\beta_x D)\Big] \\
&\quad - \sin(\beta_y W)\sinh(\beta_x W) \\
&\qquad \times \Big[D\mathrm{Ci}(\beta_x D) - D^*\mathrm{Ci}(-\beta_x D^*) + 2\pi W\Big] \\
&\quad + \cos(\beta_y W) \\
&\qquad \times \Big[\cosh(\beta_x W)(iD\mathrm{Ci}(\beta_x D) + 2W(\mathrm{Ci}(-i\beta_x W) \\
&\qquad + \mathrm{Ci}(i\beta_x W)) + iD^*\mathrm{Ci}(-\beta_x D^*)) \\
&\qquad - 2\sinh(\beta_x W)\big(2W\mathrm{Shi}(\beta_x W) + D^*\mathrm{Si}(\beta_x D^*) + D\mathrm{Si}(\beta_x D)\big)\Big]\Bigg\}\Big/ 2W
\end{aligned} \tag{82}$$

Where additionally to the functions defined above, $\mathrm{Shi}(z)$ is the hyperbolic sine integral function and $D = L + iW$. Under the assumption that $L \gg W$, this simplifies to:

$$\begin{aligned}
I_{\mathrm{d}}(\vec{\beta}) \approx \cos(\beta_y W)\Big\{& 2\,\mathrm{Chi}(|\beta_x|W)\cosh(|\beta_x|W) \\
&+ \pi\frac{L}{W}\big[\cosh(|\beta_x|W) - \sinh(|\beta_x|W)\big] \\
&- 2\,\mathrm{Shi}(|\beta_x|W)\sinh(|\beta_x|W)\Big\}
\end{aligned} \tag{83}$$

Where $\mathrm{Chi}(z)$ is the hyperbolic cosine integral function.
